# Supplementary material for: SPIDeRS: Structured Polarization for Invisible Depth and Reflectance Sensing
Source: arXiv:2312.04553 source file (2024-03-31)
Supplement: Supplementary file 1 [file tikz_supp.tex]

\begin{tikzpicture}[x=0.001\linewidth,y=0.001\linewidth,/tikzinclude/figure=addresult]
{
    \newcount\vX
    \newcount\vY
    \newcount\vdX
    \newcount\vXlabel
    \vX = 0
    \vY = 0
    \vdX = 187
    \vXlabel = -125
    \def\mysz{0.19\linewidth}

    \newcount\vdXerror
    \newcount\vdYerror
    \def\myerror#1{\normalsize \textcolor{white}{#1}}
    \def\showerror#1{
        \advance\vX by \vdXerror
        \advance\vY by \vdYerror
        \node[inner sep=0pt] (a) at (\vX,\vY) {\myerror{#1}};
        \advance\vX by -\vdXerror
        \advance\vY by -\vdYerror
    }

    \newcount\vdYbar
    \def\myszbar{0.17\linewidth}
    \def\myfontbar{\small}
    \def\putcolorbar#1#2#3{
        \vdYbar = #3
        \advance\vY by \vdYbar
        \node[inner sep=0pt, rotate=-90] (a) at (\vX,\vY){\resizebox{!}{\myszbar}{\includegraphics{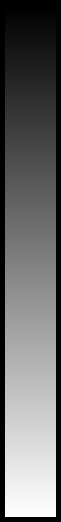}}};
        \node[inner sep=0pt, font=\myfontbar] (a) at (\vX-135,\vY) {#1};
        \node[inner sep=0pt, font=\myfontbar] (a) at (\vX+135,\vY) {#2};
        \advance\vY by -\vdYbar
        }

    \def\myfont{\normalsize}
    \vX = 0
    \node[inner sep=0pt, font=\myfont] (a) at (\vX,\vY) {RGB image};
    \advance\vX by \vdX
    \node[inner sep=0pt, font=\myfont] (a) at (\vX,\vY) {Depth};
    \advance\vX by \vdX
    \node[inner sep=0pt, font=\myfont] (a) at (\vX,\vY) {Normal};
    \advance\vX by \vdX
    \node[inner sep=0pt, font=\myfont] (a) at (\vX,\vY) {Relighting 1};
    \advance\vX by \vdX
    \node[inner sep=0pt, font=\myfont] (a) at (\vX,\vY) {Relighting 2};

    % object 1
    \vX = \vXlabel
    \advance\vY by -140
    % error position
    \vdXerror = 0
    \vdYerror = -110
    \def\myincA#1{\resizebox{\mysz}{!}{\adjincludegraphics[Clip={{0.20\width} {0.0\width} {0.25\width} {0.10\width}}]{#1}}}

    \node[inner sep=0pt, rotate=90, font=\myfont] (a) at (\vX,\vY) {\begin{tabular}{c} Structured light \\ using intensity\end{tabular}};

    \vX = 0
    \node[inner sep=0pt] (a) at (\vX,\vY) {\myincA{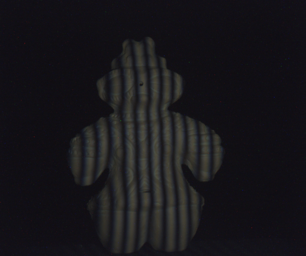}};
    \advance\vX by \vdX
    \node[inner sep=0pt] (a) at (\vX,\vY) {\myincA{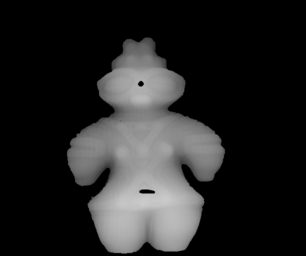}};
    \advance\vX by \vdX
    \node[inner sep=0pt] (a) at (\vX,\vY) {\myincA{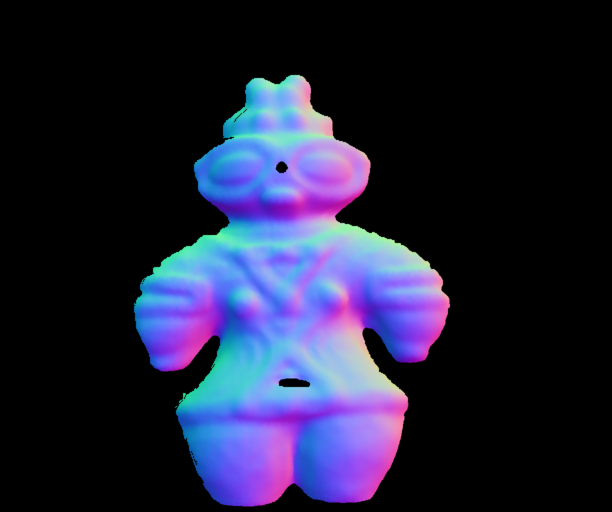}};

    \vX = \vXlabel
    \advance\vY by -250
    \node[inner sep=0pt, rotate=90, font=\myfont] (a) at (\vX,\vY) {Ours};
    \vX = 0
    \node[inner sep=0pt] (a) at (\vX,\vY) {\myincA{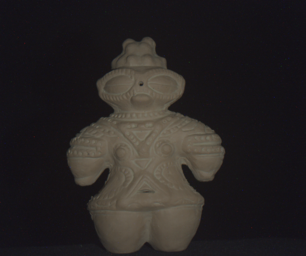}};
    \advance\vX by \vdX
    \node[inner sep=0pt] (a) at (\vX,\vY) {\myincA{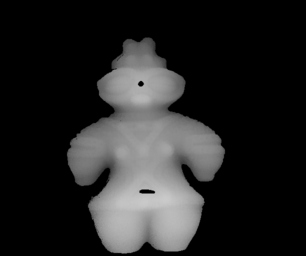}};
    \putcolorbar{450 [mm]}{490 [mm]}{-136}
    \showerror{0.38/0.28}
    \advance\vX by \vdX
    \node[inner sep=0pt] (a) at (\vX,\vY) {\myincA{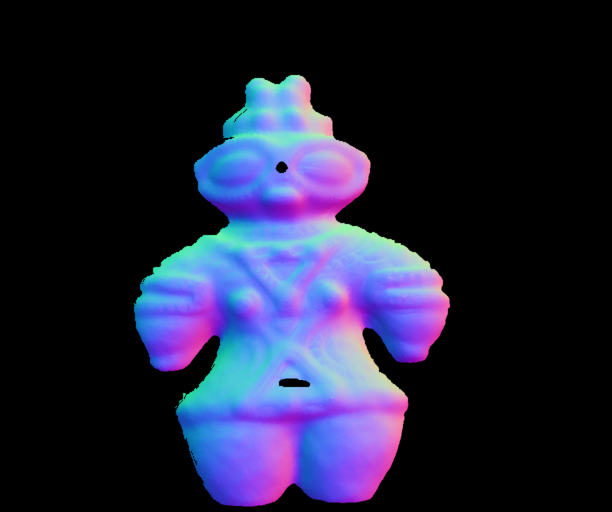}};
    \advance\vX by \vdX
    \node[inner sep=0pt] (a) at (\vX,\vY) {\myincA{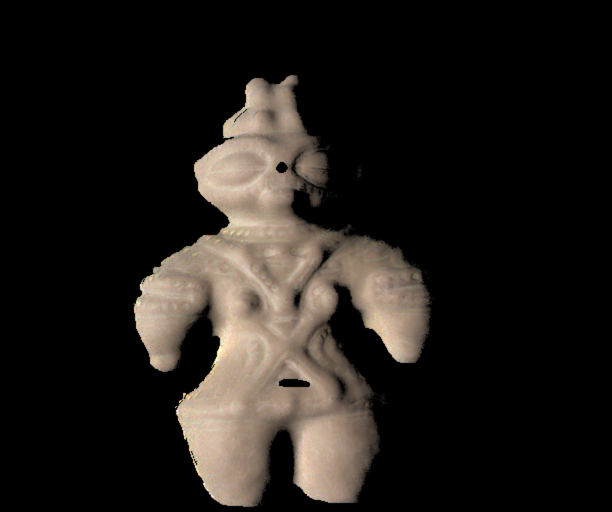}};
    \advance\vX by \vdX
    \node[inner sep=0pt] (a) at (\vX,\vY) {\myincA{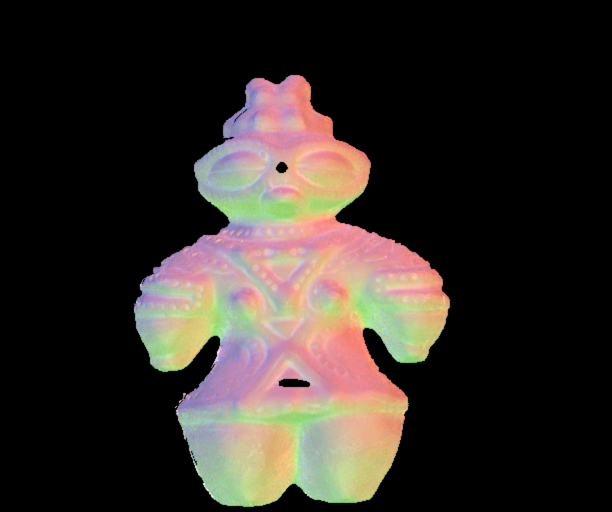}};

    % object 2
    \vX = \vXlabel
    \advance\vY by -252
    % error position
    \vdXerror = 0
    \vdYerror = -85
    \def\myincB#1{\resizebox{\mysz}{!}{\adjincludegraphics[Clip={{0.20\width} {0.0\width} {0.15\width} {0.15\width}}]{#1}}}

    \node[inner sep=0pt, rotate=90, font=\myfont] (a) at (\vX,\vY) {\begin{tabular}{c} Structured light \\ using intensity\end{tabular}};

    \vX = 0
    \node[inner sep=0pt] (a) at (\vX,\vY) {\myincB{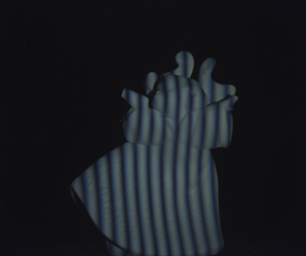}};
    \advance\vX by \vdX
    \node[inner sep=0pt] (a) at (\vX,\vY) {\myincB{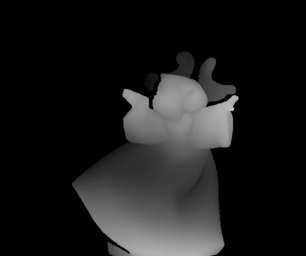}};
    \advance\vX by \vdX
    \node[inner sep=0pt] (a) at (\vX,\vY) {\myincB{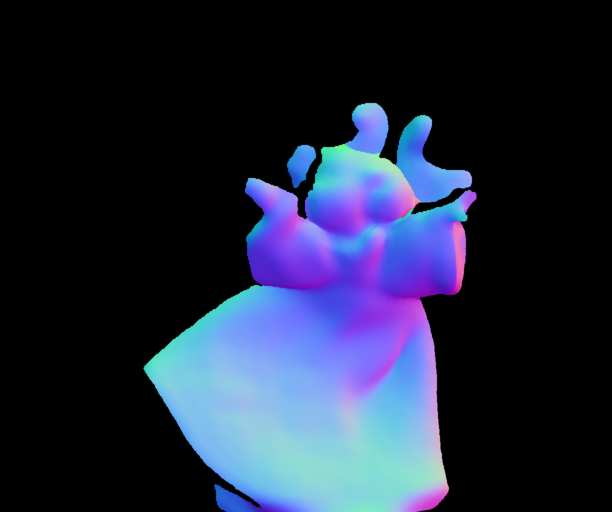}};

    \vX = \vXlabel
    \advance\vY by -198
    \node[inner sep=0pt, rotate=90, font=\myfont] (a) at (\vX,\vY) {Ours};
    \vX = 0
    \node[inner sep=0pt] (a) at (\vX,\vY) {\myincB{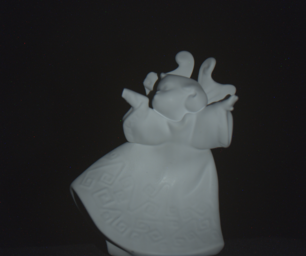}};
    \advance\vX by \vdX
    \node[inner sep=0pt] (a) at (\vX,\vY) {\myincB{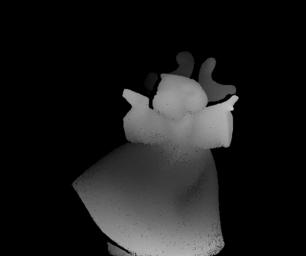}};
    \putcolorbar{430 [mm]}{480 [mm]}{-109}
    \showerror{0.73/0.53}
    \advance\vX by \vdX
    \node[inner sep=0pt] (a) at (\vX,\vY) {\myincB{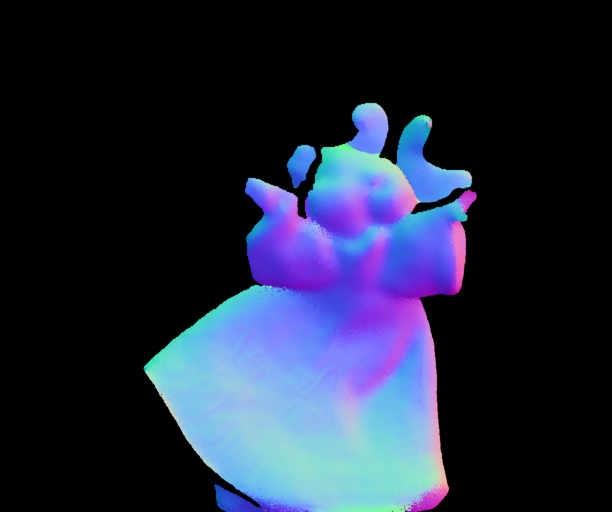}};
    \advance\vX by \vdX
    \node[inner sep=0pt] (a) at (\vX,\vY) {\myincB{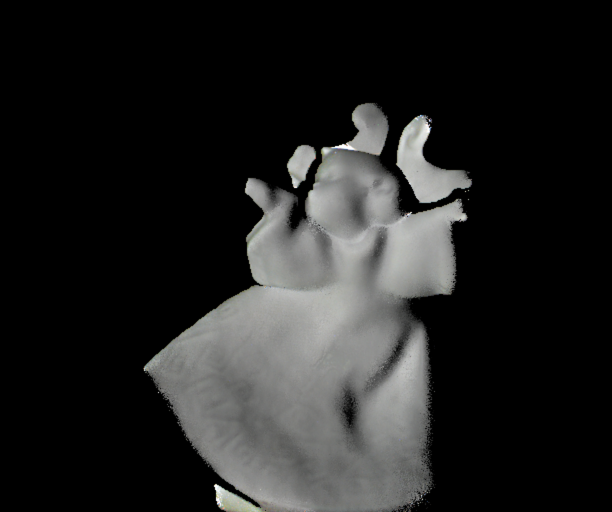}};
    \advance\vX by \vdX
    \node[inner sep=0pt] (a) at (\vX,\vY) {\myincB{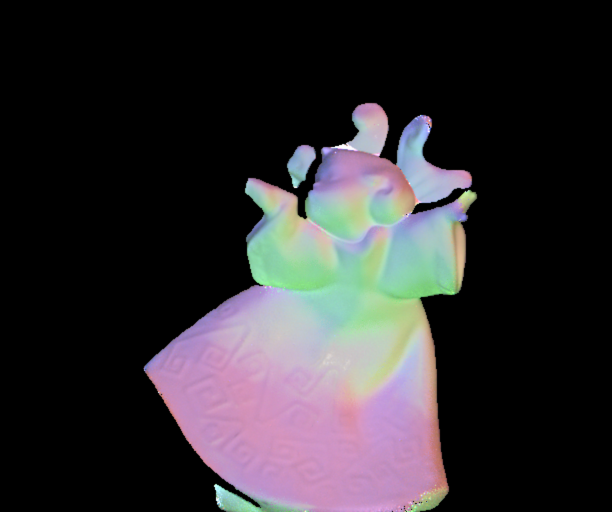}};

    % object 3
    \vX = \vXlabel
    \advance\vY by -197
    % error position
    \vdXerror = 0
    \vdYerror = -60
    \def\myincB#1{\resizebox{\mysz}{!}{\adjincludegraphics[Clip={{0.2\width} {0.1\width} {0.3\width} {0.35\width}}]{#1}}}

    \node[inner sep=0pt, rotate=90, font=\myfont] (a) at (\vX,\vY) {\begin{tabular}{c} Structured light \\ using intensity\end{tabular}};

    \vX = 0
    \node[inner sep=0pt] (a) at (\vX,\vY) {\myincB{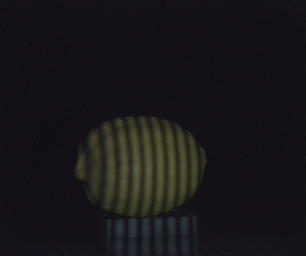}};
    \advance\vX by \vdX
    \node[inner sep=0pt] (a) at (\vX,\vY) {\myincB{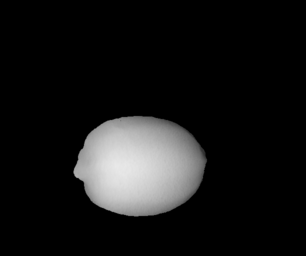}};
    \advance\vX by \vdX
    \node[inner sep=0pt] (a) at (\vX,\vY) {\myincB{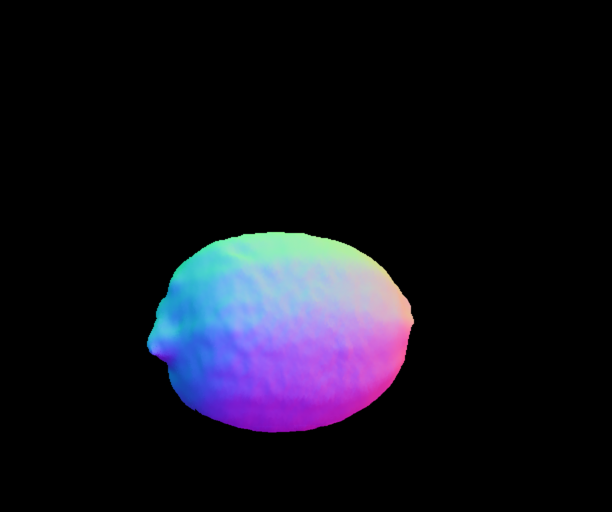}};

    \vX = \vXlabel
    \advance\vY by -140
    \node[inner sep=0pt, rotate=90, font=\myfont] (a) at (\vX,\vY) {Ours};
    \vX = 0
    \node[inner sep=0pt] (a) at (\vX,\vY) {\myincB{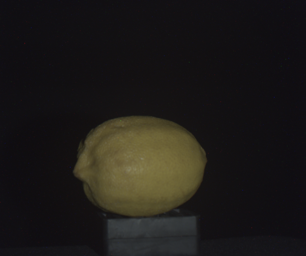}};
    \advance\vX by \vdX
    \node[inner sep=0pt] (a) at (\vX,\vY) {\myincB{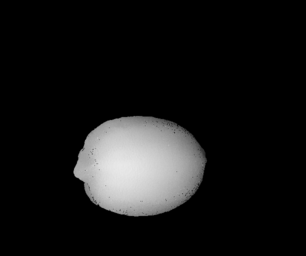}};
    \putcolorbar{440 [mm]}{490 [mm]}{-82}
    \showerror{0.68/0.50}
    \advance\vX by \vdX
    \node[inner sep=0pt] (a) at (\vX,\vY) {\myincB{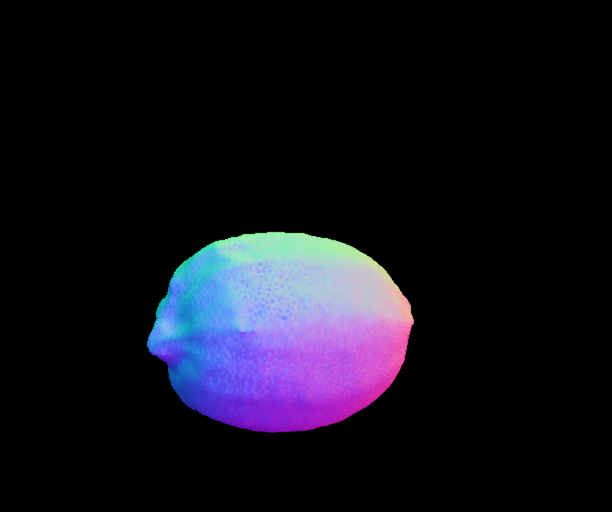}};
    \advance\vX by \vdX
    \node[inner sep=0pt] (a) at (\vX,\vY) {\myincB{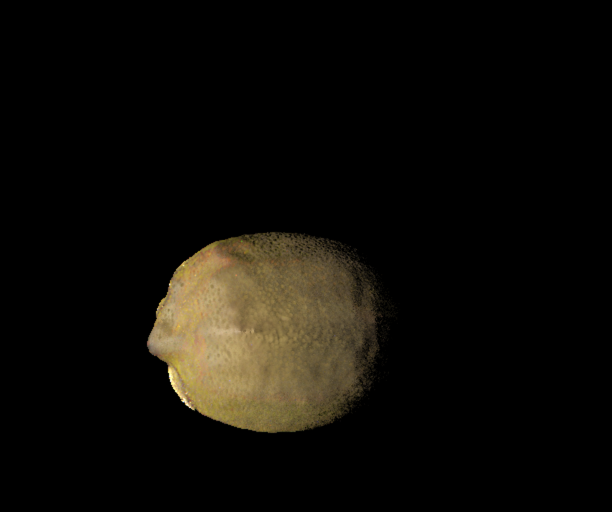}};
    \advance\vX by \vdX
    \node[inner sep=0pt] (a) at (\vX,\vY) {\myincB{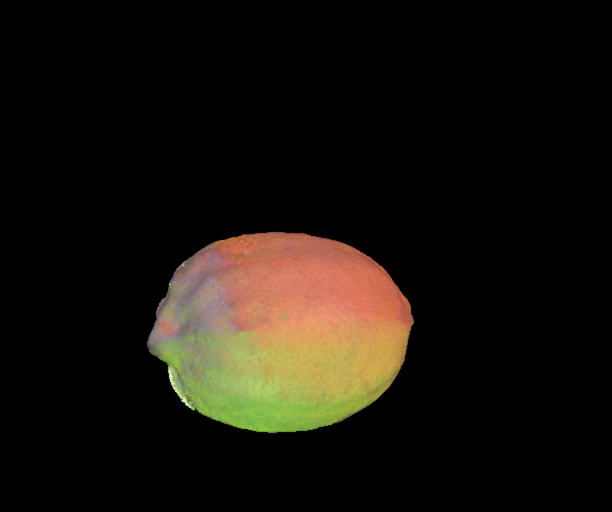}};

}
\end{tikzpicture}
